# Supplementary material for: Semantic Scene Segmentation for Robotics
Source: arXiv:2401.07589 source file (2024-01-15)
Supplement: Supplementary file 1 [file appendix12.tex]

\begin{frontmatter}
\chapter{Appendix title}%\label{chap:appa}
\end{frontmatter}

%\section{}\label{}
